# Supplementary material for: Topological Data Analysis of Ion Migration Mechanism
Source: arXiv:2303.07719 ancillary file (2023-03-14)
Supplement: Supplementary file 1 [file sato_230309_SI.pdf]

**Supporting Information**

# Topological Data Analysis of Ion Migration Mechanism

*Ryuhei Sato*[1*], *Kazuto Akagi*[1], *Shigeyuki Takagi*[2], *Kartik Sau*[1,3], *Kazuaki Kisu*[2], *Hao Li*[1], *Shin-ichi Orimo*[1,2*]

[1] *Advanced Institute for Materials Research, Tohoku University*, 2-1-1 Katahira, Aoba-ku, Sendai 980-8577, Japan

[2] *Institute for Materials Research, Tohoku University,* 2-1-1 Katahira, Aoba-ku, Sendai 980-8577, Japan.

[3]*Mathematics for Advanced Materials Open Innovation Laboratory (MathAM-OIL), National Institute of Advanced Industrial Science and Technology (AIST), c/o Advanced Institute for Materials Research (AIMR), Tohoku University*, Sendai 980-8577, Japan

**S1** ***Persistence diagram of AgI during NPT-MD simulations at various temperatures***

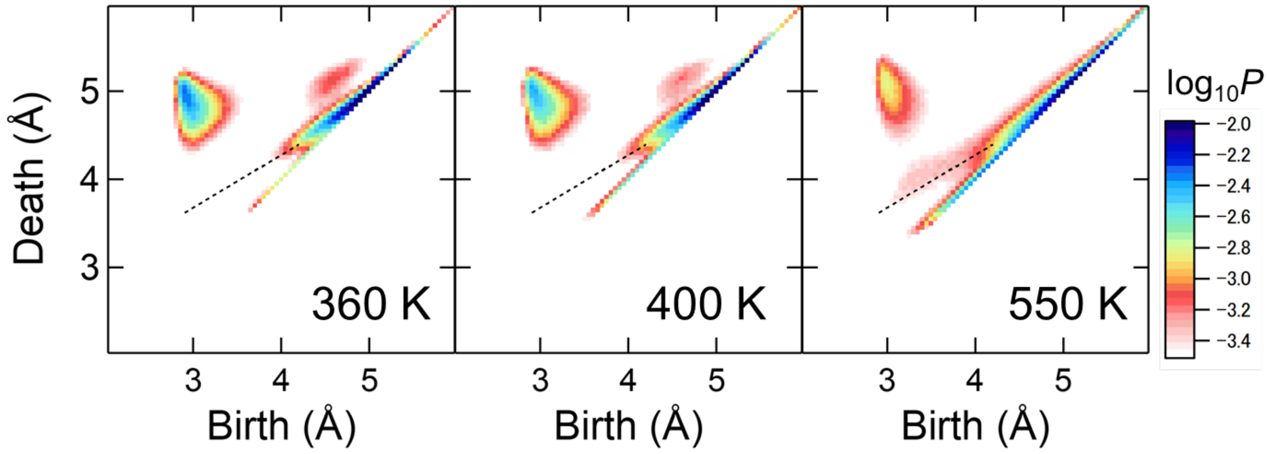


Figure S1 Time-averaged persistence diagram of the ring structure during 3-ns NPT-MD simulations of AgI for several temperatures. This persistence diagram represents a probability density distribution ($P$) normalized so that the integrated value over the squared regions [0.0, 12.0] × [0.0, 12.0] (Å$^2$) becomes unity. The color in the figure is scaled according to $\log_{10}P$ and represents the probability density per the mesh of 0.05 × 0.05 Å$^2$.

Even if the phase transition occurs, the changes in the persistence diagram with increasing ionic conductivity are comparable with that of MD simulations without phase transition. Figure S1 shows the time-averaged persistence diagram of AgI during 3-ns NPT-MD simulations. In this simulation, we employed a cubic cell, 18.8 × 16.3 × 30.5 Å, consisting of 256 Ag and I ions ($4\times2\sqrt{3}\times4$ supercell of β-AgI). The ring structures at (Birth, Death) = (2.8,4.5) and (4.2,4.4) are identical with that in the NVT-MD simulations in Fig. 3. In addition, the ring-structure distribution along the black dashed line still increases on the persistence diagrams at 550K. Note that the ring structure at around (4.6,5.1) is considered to be the specific one for β-AgI.

**S2** ***Number of atoms in each ring structure in persistence diagram at 1000K***

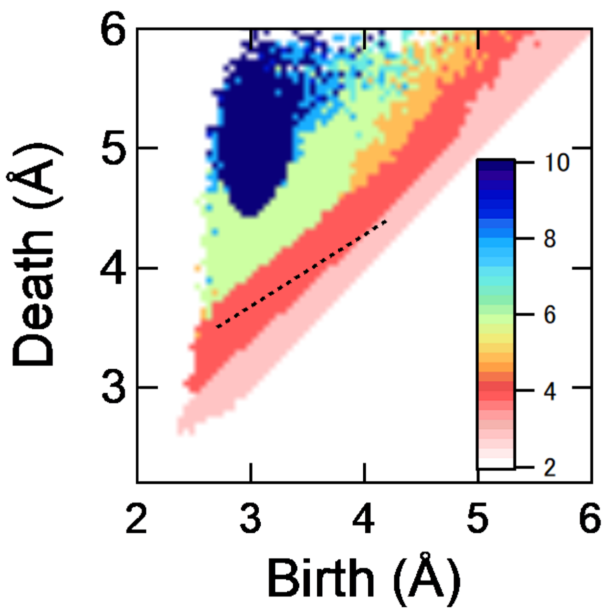


Figure S2 The distribution of most frequent number of atoms in the ring at each mesh in time-averaged persistence diagram during MD simulation for α-AgI at 1000K (most frequent numbers are calculated for each 0.05×0.05 Å mesh)

The ring structure involved in Ag ion migration consists mainly of Ag-I four-membered rings. Figure S2 shows the distribution of the most frequent number of atoms in the rings constituting each mesh in the persistence diagram for MD simulation for α-AgI at 1000K. As shown in the figure, the four-membered rings are dominant on the black dashed line, whose distribution increased when α-AgI shows superionic conductivity.

**S3** ***Bond valence analysis of four-membered rings obtained from inverse analysis***

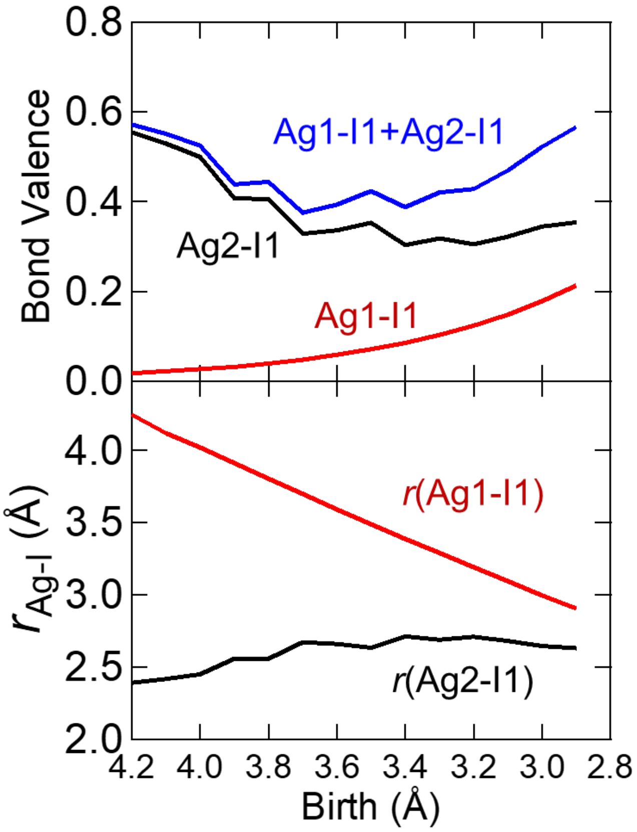


Figure S3 Change in (upper) bond valence and (lower) Ag-I distance in the four-membered ring, when it is deformed along the black dashed line in the persistence diagram at 1000K (Fig. 4(a)). The bond valence was calculated using the parameter in ref. SI1

In this Ag migration, two Ag ions in a four-membered ring interact each other via I bcc lattice. Ag2 in Fig. 4(b) moves to reduce the bond valence with I1, which correlates with the displacement of Ag1. As shown in Fig. S3 (lower), although the change in the Ag2-I1 bond distance is small, the calculated bond valence decreases largely, which compensate the increase in Ag1-I1 bond valence. In other words, the displacement of Ag2 shown by the yellow arrow in Fig. 4(b) is partly responsible for the migration of Ag1 shown by the red arrow.

**S4** ***Direction analysis of single Ag hopping***

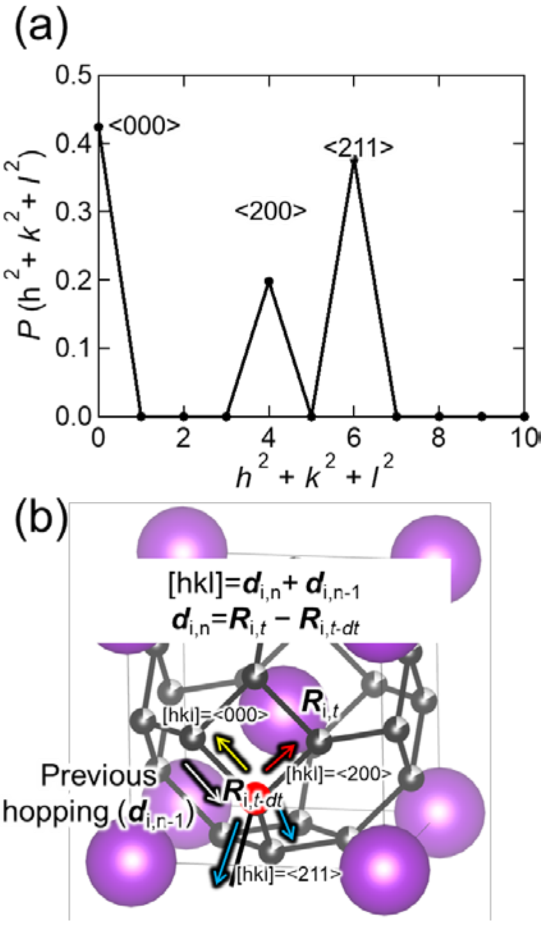


Figure S4 (a) Probability density distribution for the direction of Ag hopping between the nearest sites (between the black spheres in Fig. 1(a)) during 25-ns MD simulation for α-AgI at 1000 K. The horizontal axis $h^2+k^2+l^2$ is calculated from [hkl] = $\boldsymbol{d}_{\mathbf{i,n}}$+ $\boldsymbol{d}_{\mathbf{i,n-1}}$ using the direction of the previous n-1th hopping ($\boldsymbol{d}_{\mathbf{i,n-1}}$) and the confirmed Ag hopping direction ($\boldsymbol{d}_{\mathbf{i,n}}$) for the i-th Ag atom. Note that the position of each Ag ion is assigned to the ideal Ag stable site (a vertex of the Voronoi polyhedron of I bcc lattice) at each timestep. Here, the residence time is set to 0.05 ps. (b) Schematic diagram for α-AgI unit cell and [hkl] defined in the analysis of (a). $\boldsymbol{R}_{\mathbf{i,t}}$ in the figure represents the atomic coordinates of the nearest Ag stable site at time $t$ for the i-th Ag ion.

The probabilities of the four types of Ag migration in Fig. 5 were estimated from that of the direction of one Ag hopping during 25-ns MD simulation[SI2]; Fig. S4 shows the probability density distribution of $h^2+k^2+l^2$, the sum of squares with respect to the direction of Ag hopping migration [hkl] defined in the schematic diagram in Fig. S4(b). Note that in this analysis, each Ag ion is assigned to the stable site in Fig. 1(a) every 0.05 ps (Δt= 0.05 ps). If an Ag ion moves to another stable site after 0.05 ps, Ag hopping was considered to have occurred. The direction of hopping [hkl] is defined as [hkl] = $\boldsymbol{d}_{\mathbf{i,n}}$

+ $\boldsymbol{d}_{\mathbf{i,n-1}}$ using the direction of the previous n-1th hopping ($\boldsymbol{d}_{\mathbf{i,n-1}}$) for the i-th Ag ion and the confirmed Ag hopping direction ($\boldsymbol{d}_{\mathbf{i,n}}$). From Fig. S4(b), the direction of the backward reaction is defined as [000] in Fig. S4(a). If Ag ion migrates around the same face-centered cubic position of the unit cell, the direction is assigned as <200>, and the other two migration pathways is represented as <211>. The figure shows that Ag hopping in each direction occurs with a probability of 42% for [000], 20% for <200>, and about 38% for <211>. Note that the probability of <211> is doubled since there are two equivalent possible directions for Ag hopping (see schematic diagram in Fig. S4(b)). In previous MD simulations with a similar classical potential, the probability of the backward reaction was about 40%[SI3,SI4], and that for Ag migration to the remaining directions was about 20%[SI4], which is comparable with our result. The slight difference in the values may be caused by the difference in the setting of the residence time and temperature.

Focusing on the Ag1 hopping direction in the series of Ag migrations in Fig. 5, we find that the probability of the backward reaction (Fig. 5(a)) is 42%, and that of single Ag hopping (Fig. 5(b)) is 19%. There are two possible Ag migration with concerted motion thorough the deformation of the four-membered ring, where Ag2 hopping occurs immediately after Ag1 migration as shown in Fig, 5(c). In one Ag migration, Ag1 migrates to [200] direction, while in the other one it goes to [1-12] direction. Therefore, Ag1 hopping to these directions occurs with 39% probability. However, only Ag2 migration along [020] and [11-2] directions can change the four-membered ring shape. As a result, the probability of the concerted motion as shown in Fig. 5(c) becomes 26% ($0.39\times0.39/(1-0.42)=0.26$). The rest, 13% is explained by the concerted motion of Ag ions, in which the four-membered ring shape is maintained during Ag migration as shown in Fig. 5(d). In summary, there is a 39% probability that concerted motion of Ag ions contributes to the ion migration and this ratio is not negligible.

---

SI1 S. Adam, and J. Swenson, Migration pathways in Ag-based superionic glasses and crystals investigated by the bond valence method, *Phys. Rev. B.*, **63**, 054201, (2000).

SI2 Here, we used longer sampling time for the calculation same as the conductivity with Green-Kubo formula, because of the slow convergence. However, the obtained ring-structure hardly depends on the hopping direction, because Ag migration in any of the directions shown in Fig. 5 can be reproduced by symmetric operation of the four-membered ring deformation as in Fig. 4(b).

SI3 M. Hokazono, A. Ueda, Y. Hiwatari, Dynamical structure of superionic conductors, *Solid State Ionics*, **13**, 151-155, (1984).

SI4 P. Vashishta, and A. Rahman, Ionic Motion in α-AgI, *Phys. Rev. Lett.* **40**, 1337, (1978).
